# Supplementary material for: Rashomon Sets for Prototypical-Part Networks: Editing Interpretable Models in Real-Time
Source: arXiv:2503.01087 source file (2025-03-03)

Original Model: 12.1% confounded (182 / 1509)

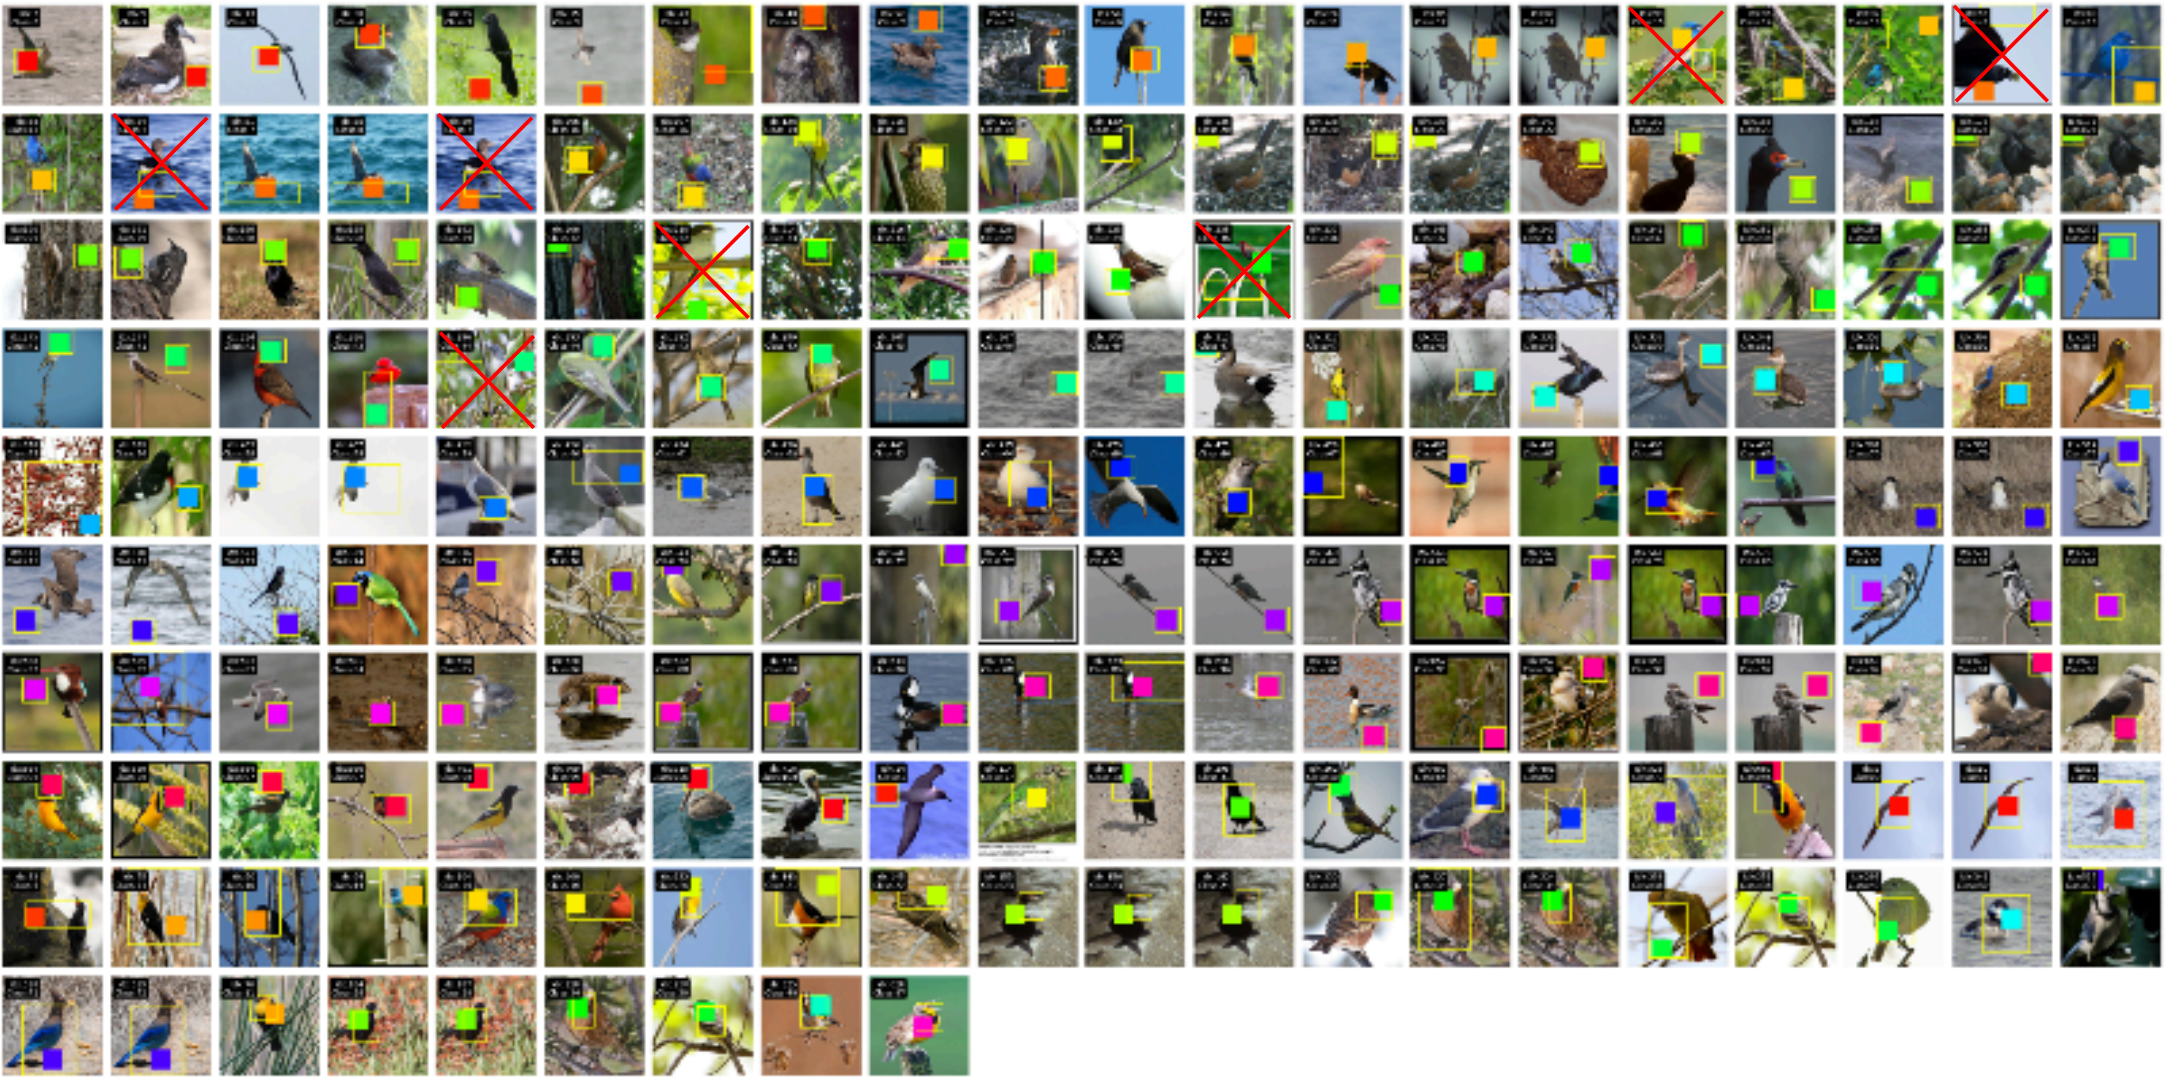

ProtoPDebug: 6.3% confounded (21 / 332)

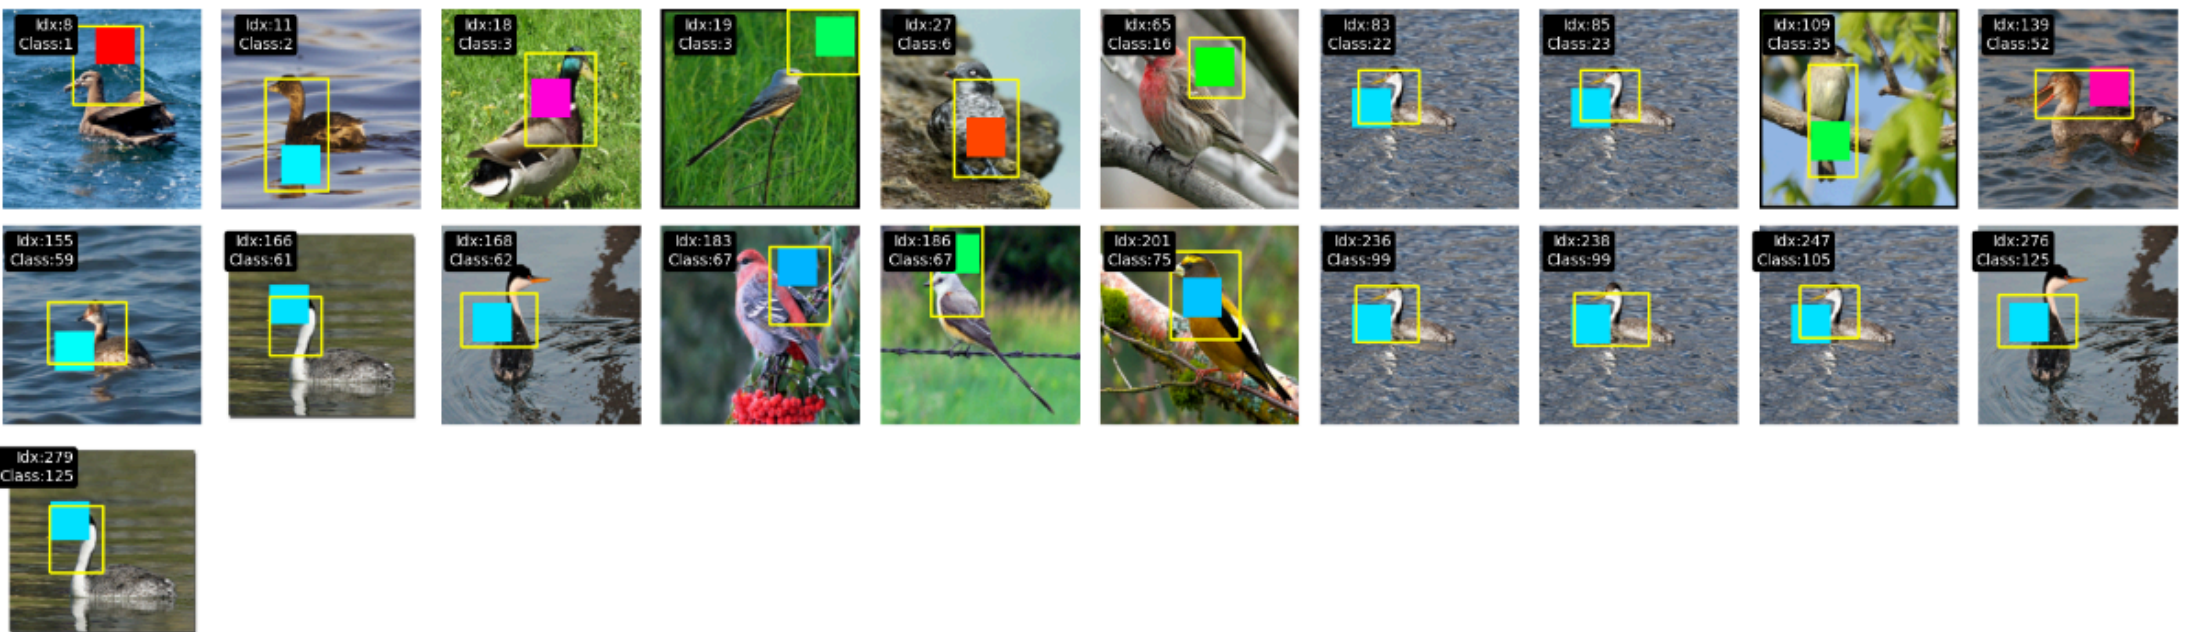

Proto-RSet: 0.5% confounded (7 / 1327)

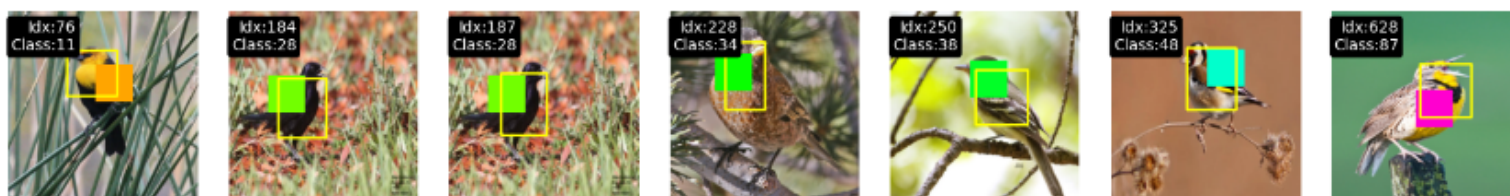



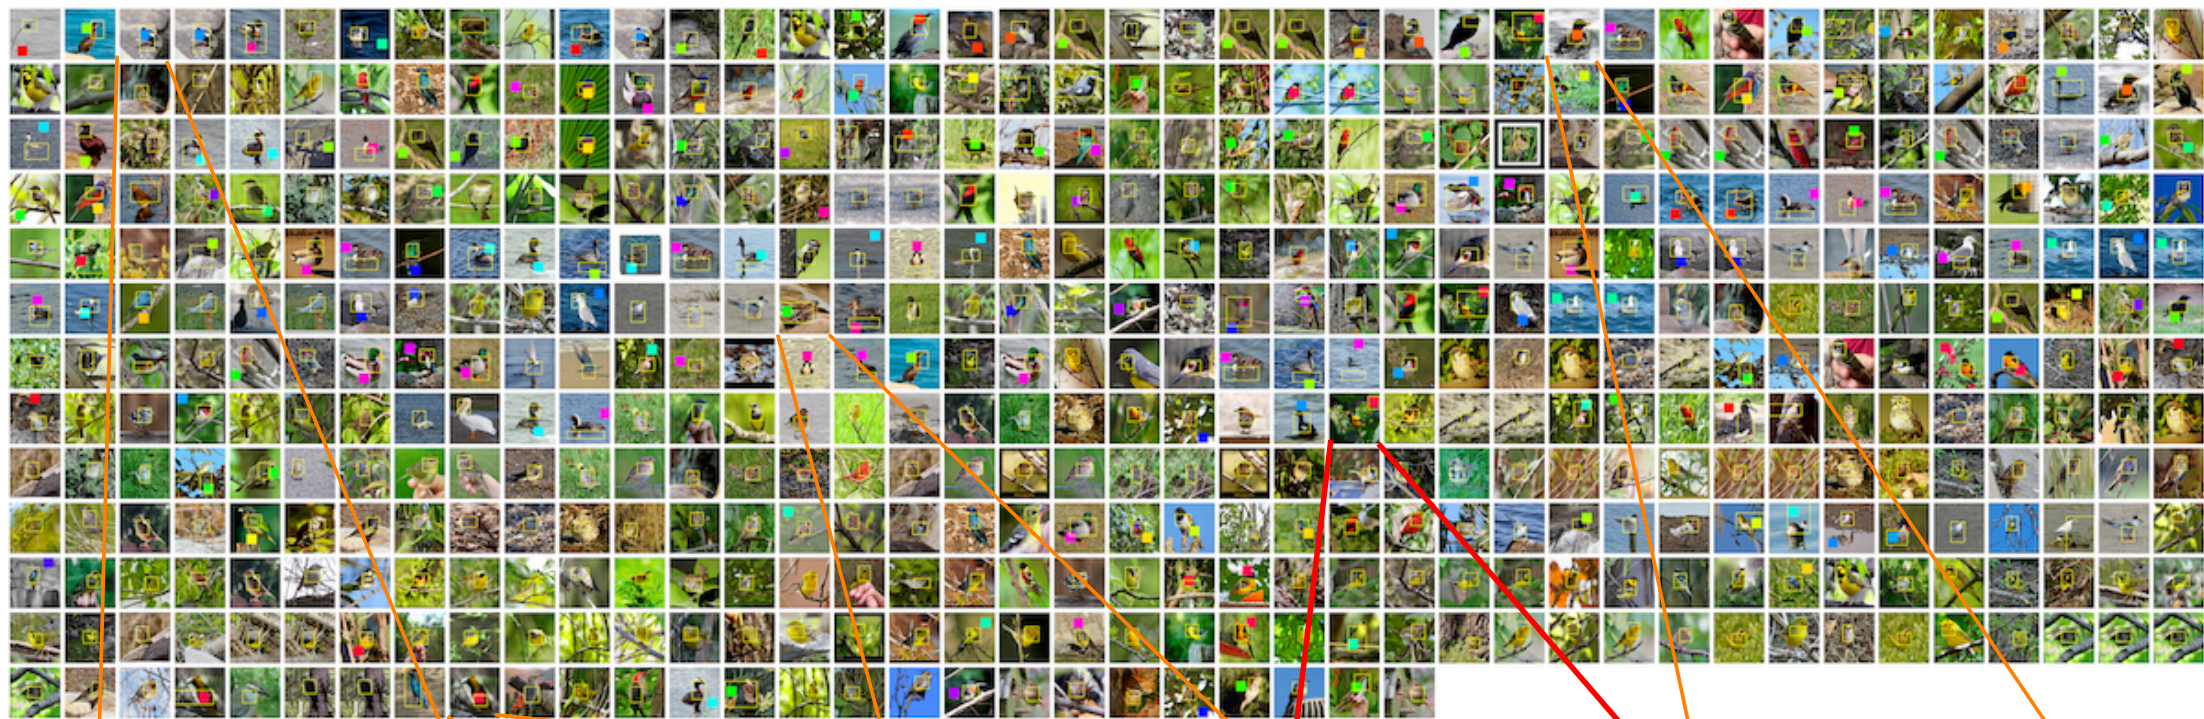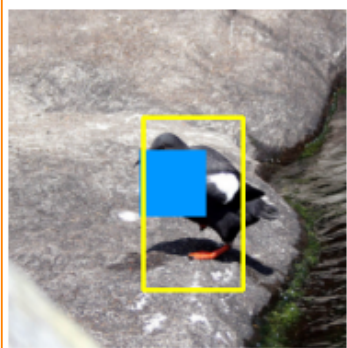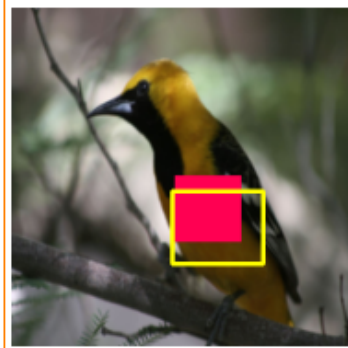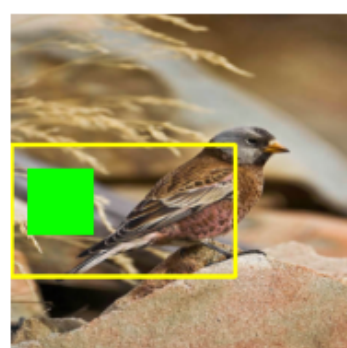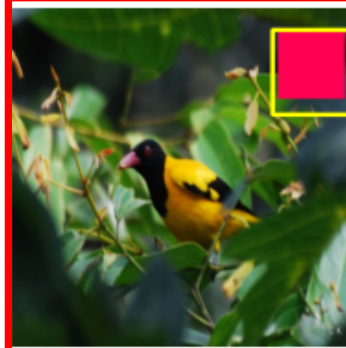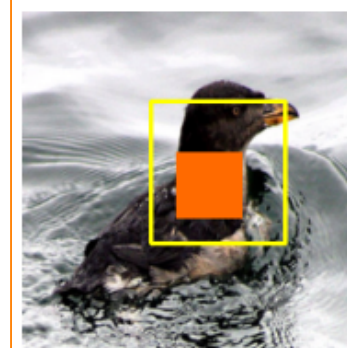

Supplement: Supplementary file 1 [file confounded-protodebug.pdf]
